# Supplementary material for: Can $GW$ Handle Multireference Systems?
Source: arXiv:2401.03745 ancillary file (2024-01-08)
Supplement: Supplementary file 1 [file si_GW4MR.pdf]

# Supplementary Material for “Can *GW* Handle Multireference Systems?”

Abdallah Ammar,<sup>1, a)</sup> Antoine Marie,<sup>1, b)</sup> Mauricio Rodríguez-Mayorga,<sup>2, c)</sup> Hugh G. A. Burton,<sup>3, d)</sup> and Pierre-François Loos<sup>1, e)</sup>

<sup>1)</sup> *Laboratoire de Chimie et Physique Quantiques (UMR 5626), Université de Toulouse, CNRS, UPS, France*

<sup>2)</sup> *Université Grenoble Alpes, CNRS, Institut NEEL, F-38042 Grenoble, France*

<sup>3)</sup> *Yusuf Hamied Department of Chemistry, University of Cambridge, Lensfield Road, Cambridge, CB2 1EW, U.K.*

## I. BE + H<sub>2</sub> REACTION

- PYSCF format of the Be(3s2p)/H(2s) basis set:

```
BASIS "ao basis" SPHERICAL PRINT
#BASIS SET: (4s) -> [2s]
H   S
    19.24060E+00      0.032828E+00
    2.899200E+00      0.231208E+00
    0.653400E+00      0.817238E+00
H   S
    0.177600E+00      1.000000E+00
#BASIS SET: (10s,3p) -> [3s,2p]
Be  S
    1267.070000E+00    0.001940E+00
    190.356000E+00    0.014786E+00
    43.295900E+00     0.071795E+00
    12.144200E+00     0.236348E+00
    3.809230E+00      0.471763E+00
    1.268470E+00      0.355183E+00
Be  S
    5.693880E+00      -0.028876E+00
    1.555630E+00      -0.177565E+00
    0.171855E+00      1.071630E+00
Be  S
    0.057181E+00      1.000000E+00
Be  P
    5.693880E+00      1.000000E+00
Be  P
    1.555630E+00      0.144045E+00
    0.171855E+00      0.949692E+00
END
```

---

<sup>a)</sup> Electronic mail: [aammar@irsamc.ups-tlse.fr](mailto:aammar@irsamc.ups-tlse.fr)

<sup>b)</sup> Electronic mail: [amarie@irsamc.ups-tlse.fr](mailto:amarie@irsamc.ups-tlse.fr)

<sup>c)</sup> Electronic mail: [marm3.14@gmail.com](mailto:marm3.14@gmail.com)

<sup>d)</sup> Electronic mail: [hgaburton@gmail.com](mailto:hgaburton@gmail.com)

<sup>e)</sup> Electronic mail: [loos@irsamc.ups-tlse.fr](mailto:loos@irsamc.ups-tlse.fr)

TABLE I. Hartree-Fock (HF) ground-state energy and the first four roots of the FCI matrix (in  $E_h$ ) for the cationic state of  $\text{BeH}_2$  as functions of  $x$  (in  $a_0$ ).

| $x$  | HF energy  | FCI energies |            |            |            |
|------|------------|--------------|------------|------------|------------|
|      |            | Root #1      | Root #2    | Root #3    | Root #4    |
| 0.00 | -15.263651 | -15.382085   | -15.325298 | -15.085238 | -15.085238 |
| 0.25 | -15.252976 | -15.371673   | -15.313744 | -15.114749 | -15.070233 |
| 0.50 | -15.237634 | -15.361208   | -15.298337 | -15.106722 | -15.060838 |
| 0.75 | -15.291210 | -15.353711   | -15.281222 | -15.106733 | -15.059047 |
| 1.00 | -15.291011 | -15.351717   | -15.264931 | -15.117632 | -15.065947 |
| 1.25 | -15.297507 | -15.355837   | -15.250765 | -15.140054 | -15.080525 |
| 1.50 | -15.308517 | -15.364227   | -15.238656 | -15.171047 | -15.099709 |
| 1.75 | -15.319927 | -15.373332   | -15.232856 | -15.200120 | -15.119700 |
| 2.00 | -15.327584 | -15.379481   | -15.257115 | -15.197410 | -15.179439 |
| 2.25 | -15.328808 | -15.380229   | -15.292627 | -15.207700 | -15.177748 |
| 2.50 | -15.322599 | -15.374630   | -15.326788 | -15.232365 | -15.164957 |
| 2.75 | -15.290361 | -15.363071   | -15.357741 | -15.253019 | -15.176695 |
| 3.00 | -15.323047 | -15.385155   | -15.347455 | -15.269897 | -15.185796 |
| 3.25 | -15.351455 | -15.409104   | -15.331626 | -15.283449 | -15.185619 |
| 3.50 | -15.375619 | -15.429384   | -15.320125 | -15.293772 | -15.216857 |
| 3.75 | -15.394136 | -15.444428   | -15.313115 | -15.299627 | -15.242929 |
| 4.00 | -15.402460 | -15.449608   | -15.303612 | -15.296734 | -15.256302 |

TABLE II. Hartree-Fock (HF) ground-state energy and the first four roots of the FCI matrix (in  $E_h$ ) for the neutral state of  $\text{BeH}_2$  as functions of  $x$  (in  $a_0$ ).

| $x$  | HF energy  | FCI energies |            |            |            |
|------|------------|--------------|------------|------------|------------|
|      |            | Root #1      | Root #2    | Root #3    | Root #4    |
| 0.00 | -15.741722 | -15.799589   | -15.544641 | -15.544641 | -15.428489 |
| 0.25 | -15.737372 | -15.794413   | -15.537486 | -15.534788 | -15.425578 |
| 0.50 | -15.727543 | -15.784419   | -15.535823 | -15.525383 | -15.427798 |
| 0.75 | -15.714324 | -15.771594   | -15.540840 | -15.519058 | -15.431159 |
| 1.00 | -15.699912 | -15.757968   | -15.552790 | -15.517841 | -15.435575 |
| 1.25 | -15.685357 | -15.744499   | -15.570455 | -15.522037 | -15.440696 |
| 1.50 | -15.670004 | -15.730657   | -15.591041 | -15.529868 | -15.445519 |
| 1.75 | -15.651879 | -15.714843   | -15.610952 | -15.538174 | -15.450125 |
| 2.00 | -15.628721 | -15.695276   | -15.626955 | -15.543742 | -15.464346 |
| 2.25 | -15.599090 | -15.671020   | -15.636897 | -15.544303 | -15.502656 |
| 2.50 | -15.562872 | -15.643185   | -15.639669 | -15.545961 | -15.538651 |
| 2.75 | -15.488827 | -15.635005   | -15.623459 | -15.575084 | -15.419795 |
| 3.00 | -15.536692 | -15.645844   | -15.623322 | -15.555947 | -15.441077 |
| 3.25 | -15.580201 | -15.680902   | -15.605617 | -15.519404 | -15.460020 |
| 3.50 | -15.618799 | -15.714004   | -15.583496 | -15.482298 | -15.476641 |
| 3.75 | -15.650408 | -15.741386   | -15.559087 | -15.489482 | -15.463372 |
| 4.00 | -15.669900 | -15.757444   | -15.533429 | -15.493812 | -15.474227 |

TABLE III. Hartree-Fock (HF) ground-state energy and the first four roots of the FCI matrix (in  $E_h$ ) for the anionic state of  $\text{BeH}_2$  as functions of  $x$  (in  $a_0$ ).

| $x$  | HF energy  | FCI energies |            |            |            |
|------|------------|--------------|------------|------------|------------|
|      |            | Root #1      | Root #2    | Root #3    | Root #4    |
| 0.00 | -15.603945 | -15.665746   | -15.665745 | -15.637509 | -15.488977 |
| 0.25 | -15.609962 | -15.669333   | -15.658440 | -15.618335 | -15.466462 |
| 0.50 | -15.618880 | -15.676885   | -15.647558 | -15.588419 | -15.434329 |
| 0.75 | -15.626063 | -15.683328   | -15.634960 | -15.557903 | -15.427763 |
| 1.00 | -15.631893 | -15.688793   | -15.622295 | -15.530885 | -15.459442 |
| 1.25 | -15.636212 | -15.693052   | -15.610177 | -15.508412 | -15.494663 |
| 1.50 | -15.637743 | -15.694952   | -15.597893 | -15.530887 | -15.488922 |
| 1.75 | -15.634550 | -15.692845   | -15.583787 | -15.565031 | -15.507572 |
| 2.00 | -15.624821 | -15.685217   | -15.594389 | -15.566038 | -15.525504 |
| 2.25 | -15.607503 | -15.671167   | -15.617303 | -15.543518 | -15.538060 |
| 2.50 | -15.582541 | -15.650743   | -15.633228 | -15.544405 | -15.516656 |
| 2.75 | -15.550948 | -15.642510   | -15.625031 | -15.544398 | -15.493360 |
| 3.00 | -15.569582 | -15.646204   | -15.596108 | -15.538431 | -15.510903 |
| 3.25 | -15.568183 | -15.645988   | -15.566798 | -15.543336 | -15.527228 |
| 3.50 | -15.564771 | -15.644185   | -15.574534 | -15.542739 | -15.511569 |
| 3.75 | -15.563476 | -15.642923   | -15.600813 | -15.561380 | -15.514386 |
| 4.00 | -15.564207 | -15.640040   | -15.616411 | -15.587029 | -15.508473 |

## II. MULTIREFERENCE SYSTEMS

TABLE IV. FCI and CCSD(T) ground-state energies (in  $E_h$ ) for the cationic, neutral, and anionic states of the multireference systems considered in this study. The Hartree-Fock ground-state energy (solution #1) of the neutral state is also reported.

| System         | HF energy | FCI energies |           |           | CCSD(T) energies |           |           |
|----------------|-----------|--------------|-----------|-----------|------------------|-----------|-----------|
|                |           | Cation       | Neutral   | Anion     | Cation           | Neutral   | Anion     |
| B <sub>2</sub> | −49.0422  | −48.9484     | −49.2781  | −49.3465  | −48.9461         | −49.2699  | −49.3430  |
| LiF            | −106.9856 | −106.8850    | −107.3012 | −107.3021 | −106.9039        | −107.3201 | −107.3209 |
| BeO            | −89.4427  | −89.3772     | −89.7435  | −89.8159  | −89.3767         | −89.7421  | −89.8146  |
| BN             | −78.9085  | −78.8315     | −79.2698  | −79.3797  | −78.8293         | −79.2697  | −79.3754  |
| C <sub>2</sub> | −75.4036  | −75.3291     | −75.7866  | −75.8968  | −75.3274         | −75.7845  | −75.8945  |
| O <sub>3</sub> | −224.3521 | −224.6858    | −225.1480 | −225.1951 | −224.6750        | −225.1419 | −225.1926 |

TABLE V. Principal IP, principal EA, and fundamental gap (in eV) for a selection of multireference systems computed at the  $G_0W_0$  level with different starting points (HF, BLYP, B3LYP, CAM-B3LYP) with the def2-TZVPP basis. The error with respect to the reference FCI value is reported in parentheses. See the main manuscript for more details.

| Mol.           |     | $G_0W_0$     |              |              |              | FCI   |
|----------------|-----|--------------|--------------|--------------|--------------|-------|
|                |     | HF(#1)       | BLYP         | B3LYP        | CAM-B3LYP    |       |
| B <sub>2</sub> | IP  | 9.06(+0.09)  | 8.61(−0.36)  | 8.58(−0.39)  | 8.80(−0.17)  | 8.97  |
|                | EA  | 2.05(+0.19)  | 2.22(+0.36)  | 2.36(+0.50)  | 2.13(+0.27)  | 1.86  |
|                | Gap | 7.01(−0.11)  | 6.39(−0.72)  | 6.23(−0.88)  | 6.66(−0.45)  | 7.11  |
| LiF            | IP  | 11.31(−0.01) | 9.65(−1.67)  | 10.45(−0.87) | 11.11(−0.22) | 11.32 |
|                | EA  | 0.01(−0.01)  | 0.25(+0.23)  | 0.18(+0.16)  | 0.07(+0.05)  | 0.02  |
|                | Gap | 11.29(−0.01) | 9.90(−1.40)  | 10.62(−0.68) | 11.18(−0.12) | 11.30 |
| BeO            | IP  | 9.76(−0.21)  | 9.46(−0.51)  | 9.38(−0.59)  | 9.84(−0.13)  | 9.97  |
|                | EA  | 2.09(+0.12)  | 1.66(−0.31)  | 2.05(+0.08)  | 1.97(+0.00)  | 1.97  |
|                | Gap | 7.67(−0.32)  | 7.81(+0.19)  | 7.34(−0.56)  | 7.88(−0.12)  | 8.00  |
| BN             | IP  | 11.69(−0.24) | 10.79(−1.14) | 11.29(−0.64) | 11.57(−0.36) | 11.93 |
|                | EA  | 3.83(+0.84)  | 3.82(+0.82)  | 3.63(+0.64)  | 3.53(+0.54)  | 2.99  |
|                | Gap | 7.86(−1.08)  | 6.97(−1.97)  | 7.66(−1.28)  | 8.03(−0.91)  | 8.94  |
| C <sub>2</sub> | IP  | 12.92(+0.48) |              | 12.22(−0.23) | 12.47(+0.02) | 12.45 |
|                | EA  | 4.08(+1.08)  |              | 3.96(+0.96)  | 3.88(+0.88)  | 3.00  |
|                | Gap | 8.85(−0.60)  |              | 8.26(−1.19)  | 8.59(−0.86)  | 9.45  |
| O <sub>3</sub> | IP  | 13.50(+0.92) | 11.79(−0.79) | 12.26(−0.32) | 12.80(+0.22) | 12.58 |
|                | EA  | 1.96(+0.68)  | 1.96(+0.68)  | 1.96(+0.68)  | 1.98(+0.70)  | 1.28  |
|                | Gap | 11.54(+0.25) | 9.82(−1.47)  | 10.30(−0.99) | 10.82(−0.47) | 11.29 |

The  $G_0W_0$  results computed with Kohn-Sham (KS) starting points for the multireference molecules studied in the main manuscript are reported in Table V. First of all, the stability analysis reveals that all density-functional approximations employed here lead to one stable restricted solution only. The performance of  $G_0W_0$ @KS shows that only  $G_0W_0$ @CAM-B3LYP produces competitive IPs, EAs, and gaps when compared to the  $G_0W_0$ @HF(#1) results. Notably, substantial errors of approximately 0.9 eV in gaps can still arise. It is noteworthy to mention that, for C<sub>2</sub>, the BLYP KS determinant exhibits a non-Aufbau filling, rendering it impossible to compute the  $G_0W_0$  correction. One way to eschew this difficulty is to rely on the Tamm–Dancoff approximation for the computation of the polarizability but we have not pursued this possibility here.

### III. TRIANGULAR-SHAPED $H_6$ CLUSTER

- Geometry of the  $H_6$  cluster with triangular arrangement (in Å):

|   |               |               |               |
|---|---------------|---------------|---------------|
| H | 0.00000000000 | 0.00000000000 | 0.00000000000 |
| H | 1.00000000000 | 1.73205080757 | 0.00000000000 |
| H | 2.00000000000 | 0.00000000000 | 0.00000000000 |
| H | 3.00000000000 | 1.73205080757 | 0.00000000000 |
| H | 4.00000000000 | 0.00000000000 | 0.00000000000 |
| H | 2.00000000000 | 3.46410161514 | 0.00000000000 |

#### IV. DISSOCIATION CURVE OF HF

TABLE VI. IPs (in eV) of the HF molecule as a function of the internuclear distance  $R_{\text{H-F}}$  (in Å) computed at various levels of theory with the cc-pVDZ basis set.

| $R_{\text{H-F}}$ | FCI   | RHF   | UHF   | $G_0W_0\text{@RHF}$ | $G_0W_0\text{@UHF}$ | qsGW@RHF | qsGW@UHF |
|------------------|-------|-------|-------|---------------------|---------------------|----------|----------|
| 0.50             | 17.29 | 18.62 | 18.62 | 17.26               | 17.26               | 17.39    | 17.39    |
| 0.55             | 17.06 | 18.40 | 18.40 | 17.05               | 17.05               | 17.17    | 17.17    |
| 0.60             | 16.84 | 18.20 | 18.20 | 16.84               | 16.84               | 16.95    | 16.95    |
| 0.65             | 16.61 | 18.00 | 18.00 | 16.63               | 16.63               | 16.73    | 16.73    |
| 0.70             | 16.39 | 17.81 | 17.81 | 16.41               | 16.41               | 16.52    | 16.52    |
| 0.75             | 16.16 | 17.63 | 17.63 | 16.20               | 16.20               | 16.30    | 16.30    |
| 0.80             | 15.94 | 17.46 | 17.46 | 16.00               | 16.00               | 16.09    | 16.10    |
| 0.85             | 15.72 | 17.31 | 17.31 | 15.79               | 15.79               | 15.90    | 15.90    |
| 0.90             | 15.51 | 17.16 | 17.16 | 15.60               | 15.60               | 15.70    | 15.70    |
| 0.95             | 15.31 | 17.03 | 17.03 | 15.41               | 15.41               | 15.52    | 15.52    |
| 1.00             | 15.11 | 16.90 | 16.90 | 15.24               | 15.24               | 15.35    | 15.35    |
| 1.05             | 14.92 | 16.79 | 16.79 | 15.06               | 15.06               | 15.19    | 15.19    |
| 1.10             | 14.74 | 16.69 | 16.69 | 14.90               | 14.90               | 15.04    | 15.04    |
| 1.15             | 14.57 | 16.60 | 16.60 | 14.75               | 14.75               | 14.91    | 14.91    |
| 1.20             | 14.40 | 16.52 | 16.52 | 14.60               | 14.60               | 14.78    | 14.78    |
| 1.25             | 14.25 | 16.45 | 16.45 | 14.46               | 14.46               | 14.66    | 14.66    |
| 1.30             | 14.11 | 16.38 | 16.24 | 14.32               | 14.31               | 14.54    | 14.54    |
| 1.35             | 13.98 | 16.32 | 15.34 | 14.20               | 14.54               | 14.44    | 14.44    |
| 1.40             | 13.86 | 16.02 | 14.95 | 14.07               | 14.81               | 14.35    | 14.35    |
| 1.45             | 13.75 | 15.69 | 14.71 | 13.96               | 15.06               | 14.26    | 14.26    |
| 1.50             | 13.65 | 15.38 | 14.53 | 13.84               | 14.83               | 14.17    | 14.17    |
| 1.55             | 13.57 | 15.08 | 14.40 | 13.74               | 14.59               | 14.10    | 14.08    |
| 1.60             | 13.50 | 14.80 | 14.30 | 13.63               | 14.39               | 14.02    | 14.12    |
| 1.65             | 13.43 | 14.53 | 14.22 | 13.53               | 14.22               | 13.95    | 14.31    |
| 1.70             | 13.38 | 14.28 | 14.15 | 13.44               | 14.09               | 13.89    | 14.38    |
| 1.75             | 13.34 | 14.04 | 14.09 | 13.34               | 13.98               | 13.82    | 14.21    |
| 1.80             | 13.31 | 13.82 | 14.04 | 13.25               | 13.90               | 13.77    | 14.05    |
| 1.85             | 13.29 | 13.61 | 14.00 | 13.16               | 13.83               | 13.71    | 13.91    |
| 1.90             | 13.27 | 13.41 | 13.96 | 13.08               | 13.77               | 13.65    | 13.80    |
| 1.95             | 13.26 | 13.21 | 13.93 | 12.99               | 13.72               | 13.60    | 13.71    |
| 2.00             | 13.26 | 13.03 | 13.90 | 12.91               | 13.69               | 13.55    | 13.65    |
| 2.05             | 13.26 | 12.86 | 13.88 | 12.83               | 13.66               | 13.50    | 13.60    |
| 2.10             | 13.27 | 12.70 | 13.86 | 12.76               | 13.63               | 13.46    | 13.57    |
| 2.15             | 13.28 | 12.54 | 13.84 | 12.68               | 13.61               | 13.38    | 13.55    |
| 2.20             | 13.30 | 12.39 | 13.82 | 12.61               | 13.60               | 13.27    | 13.53    |
| 2.25             | 13.31 | 12.25 | 13.80 | 12.54               | 13.58               | 13.17    | 13.52    |
| 2.30             | 13.33 | 12.11 | 13.79 | 12.48               | 13.57               | 13.07    | 13.51    |
| 2.35             | 13.34 | 11.98 | 13.78 | 12.41               | 13.56               | 12.98    | 13.51    |
| 2.40             | 13.36 | 11.86 | 13.77 | 12.30               | 13.55               | 12.89    | 13.50    |
| 2.45             | 13.38 | 11.74 | 13.75 | 12.20               | 13.54               | 12.80    | 13.50    |
| 2.50             | 13.39 | 11.62 | 13.75 | 12.11               | 13.54               | 12.72    | 13.50    |
| 2.55             | 13.40 | 11.51 | 13.74 | 12.01               | 13.53               | 12.64    | 13.49    |
| 2.60             | 13.42 | 11.41 | 13.73 | 11.93               | 13.53               | 12.57    | 13.49    |
| 2.65             | 13.43 | 11.31 | 13.72 | 11.85               | 13.52               | 12.50    | 13.49    |
| 2.70             | 13.44 | 11.21 | 13.71 | 11.77               | 13.52               | 12.43    | 13.49    |
| 2.75             | 13.46 | 11.12 | 13.71 | 11.69               | 13.51               | 12.37    | 13.49    |
| 2.80             | 13.47 | 11.03 | 13.70 | 11.62               | 13.51               | 12.31    | 13.48    |
| 2.85             | 13.48 | 10.95 | 13.70 | 11.55               | 13.50               | 12.25    | 13.48    |
| 2.90             | 13.48 | 10.86 | 13.69 | 11.49               | 13.50               | 12.19    | 13.48    |
| 2.95             | 13.49 | 10.79 | 13.68 | 11.43               | 13.50               | 12.14    | 13.48    |
| 3.00             | 13.50 | 10.71 | 13.68 | 11.37               | 13.49               | 12.09    | 13.48    |
| 3.05             | 13.51 | 10.64 | 13.68 | 11.31               | 13.49               | 12.04    | 13.47    |
| 3.10             | 13.51 | 10.57 | 13.67 | 11.26               | 13.49               | 12.00    | 13.47    |
| 3.15             | 13.52 | 10.50 | 13.67 | 11.21               | 13.49               | 11.95    | 13.47    |
| 3.20             | 13.52 | 10.44 | 13.66 | 11.16               | 13.48               | 11.91    | 13.47    |
| 3.25             | 13.53 | 10.38 | 13.66 | 11.12               | 13.48               | 11.87    | 13.47    |
| 3.30             | 13.53 | 10.32 | 13.66 | 11.07               | 13.48               | 11.83    | 13.46    |
| 3.35             | 13.53 | 10.26 | 13.65 | 11.03               | 13.48               | 11.80    | 13.46    |
| 3.40             | 13.54 | 10.21 | 13.65 | 10.99               | 13.47               | 11.76    | 13.46    |
| 3.45             | 13.54 | 10.15 | 13.65 | 10.96               | 13.47               | 11.73    | 13.46    |
| 3.50             | 13.54 | 10.10 | 13.65 | 10.92               | 13.47               | 11.70    | 13.46    |

**ACKNOWLEDGMENTS**

This project has received financial support from the European Research Council (ERC) under the European Union's Horizon 2020 research and innovation programme (Grant agreement No. 863481) for funding.
